# Supplementary material for: Everywhere Learning: Artificial Intelligence with Pointwise Constraints
Source: arXiv:2606.01557 source file (2026-10-02)
Supplement: Supplementary file 1 [file gnns.tex]

\subsection{Workflow Performance Prediction: Experimental Details}
\label{app:coding_af_details}

We evaluate pointwise-constrained training on the Coding-AF portion of
FLORA-Bench. The benchmark contains agentic workflows evaluated on two code
generation datasets, MBPP and HumanEval. Each example consists of a programming
task, an agentic workflow represented as a computational graph, and a binary
label indicating whether the workflow successfully solves the task.

\textbf{Architecture.}
We use the graph neural network predictor from FLORA-Bench. Workflow nodes are
represented using 384-dimensional sentence-transformer embeddings. A two-layer
graph convolutional network with GCNConv layers encodes the workflow graph,
after which node representations are aggregated using global mean pooling. The
task embedding is projected into the same latent space and concatenated with the
pooled workflow representation. An MLP followed by a sigmoid produces the
predicted probability
\begin{equation}
    p_\theta(z_i) \in (0,1),
\end{equation}
where \(z_i\) denotes the task--workflow pair and \(\theta\) denotes all trainable
model parameters. We use a hidden dimension of \(2048\) and dropout probability
\(0.08\).

For a labeled training example \((z_i,y_i)\), its binary cross-entropy loss is
\begin{equation}
    b_i(\theta)
    =
    -y_i\log p_\theta(z_i)
    -(1-y_i)\log\!\left(1-p_\theta(z_i)\right).
\end{equation}

\textbf{ERM baseline.}
The empirical-risk minimization baseline minimizes the batch-mean binary
cross-entropy,
\begin{equation}
    \min_\theta
    \quad
    \frac{1}{n}
    \sum_{i=1}^{n} b_i(\theta).
    \label{eq:coding_erm}
\end{equation}
This baseline uses the same architecture, optimizer, data splits, and model
selection procedure as the constrained methods.

\textbf{Pointwise constraints.}
We next associate an individual loss constraint with every training example:
\begin{align}
    \min_\theta
    \quad&
    \frac{1}{n}\sum_{i=1}^{n} b_i(\theta)
    \label{eq:coding_pointwise_primal}\\
    \text{s.t.}\quad&
    b_i(\theta)\leq \tau,
    \qquad i=1,\ldots,n.
    \nonumber
\end{align}
Here, \(\tau\) is a common per-example BCE tolerance. Defining
\begin{equation}
    g_i(\theta)=b_i(\theta)-\tau,
\end{equation}
the Lagrangian used during training is
\begin{equation}
    \mathcal{L}(\theta,\lambda)
    =
    \frac{1}{n}\sum_{i=1}^{n}b_i(\theta)
    +
    \sum_{i=1}^{n}\lambda_i g_i(\theta),
    \qquad
    \lambda_i\geq 0.
    \label{eq:coding_lagrangian}
\end{equation}
Thus, every training example has its own nonnegative dual variable
\(\lambda_i\). Examples whose losses remain above the tolerance receive
increasingly large multipliers and consequently exert greater influence on
subsequent parameter updates.

The Pointwise method performs projected dual-ascent updates
\begin{equation}
    \lambda_i
    \leftarrow
    \left[
        \lambda_i+\eta_\lambda g_i(\theta)
    \right]_+,
    \label{eq:coding_pointwise_update}
\end{equation}
where \([a]_+=\max\{a,0\}\). No upper bound is imposed on the Pointwise
multipliers.

\textbf{Clipped pointwise constraints.}
The Clipped method uses the same primal loss and pointwise constraints but
restricts every dual variable to the interval
\begin{equation}
    0\leq\lambda_i\leq\gamma.
\end{equation}
Its dual update is therefore
\begin{equation}
    \lambda_i
    \leftarrow
    \operatorname{clip}
    \left(
        \lambda_i+\eta_\lambda g_i(\theta),
        0,\gamma
    \right).
    \label{eq:coding_clipped_update}
\end{equation}
We set \(\gamma=1\) for the numerical result shown in the main body.

\textbf{Tolerance selection.}
The constraint tolerance is selected separately for each random seed. We first
train the ERM model and record its per-example BCE values on the training set.
We then set
\begin{equation}
    \tau
    =
    Q_{0.75}
    \left(
        \left\{
            b_i(\widehat{\theta}_{\mathrm{ERM}})
        \right\}_{i=1}^{n}
    \right),
    \label{eq:coding_tolerance}
\end{equation}
where \(Q_{0.75}\) denotes the linearly interpolated empirical \(75\)-th
percentile. The corresponding Pointwise and Clipped runs for that seed use the
same value of \(\tau\). Consequently, their constraint violations
\(g_i=b_i-\tau\) are directly comparable.

\textbf{Optimization and model selection.}
All three methods are trained for \(280\) epochs using Adam with initial learning
rate \(2\times10^{-5}\), weight decay \(1\times10^{-4}\), and batch size \(512\).
We use cosine learning-rate decay with a minimum learning rate of
\(5\times10^{-6}\). Validation is performed after every epoch, and the checkpoint
with the highest validation accuracy is retained for test evaluation.

For Pointwise and Clipped training, the dual learning rate is
\(\eta_\lambda=1\). The multipliers are initialized to \(1/512\), matching the
inverse batch size. Dual updates are disabled for the first \(120\) global
optimization steps and are then performed after every training batch. The ERM
baseline does not use the dual term or update per-example multipliers.

\textbf{Evaluation.}
Models are trained on the Coding-AF training split and evaluated separately on
the MBPP and HumanEval test subsets. We report test binary cross-entropy and
classification accuracy, using a probability threshold of \(0.5\) for the
binary predictions. For each method and dataset, the bars show the mean across
random seeds, and the error bars show one standard deviation.

The constraint-violation plots use
\begin{equation}
    g_i=b_i-\tau
\end{equation}
and aggregate the empirical distributions across seeds. For ERM, the tolerance
used to center these distributions is taken from the constrained run with the
same seed, ensuring that ERM, Pointwise, and Clipped violations are displayed
relative to the same seed-specific threshold.
